# Supplementary material for: Multiparty Classical Choreographies
Source: arXiv:1808.05088 source file (2018-12-02)
Supplement: Supplementary file 1 [file appendix.tex]

\section{Appendix}\label{sec:app}

In this Appendix, we discuss main proof-theoretic tranformations used
in the system: ones giving rise to commuting conversions (see
Figs.~\ref{fig:commconv_action} and~\ref{fig:commuting}), evaluation
rules (see Figs.~\ref{fig:action_semantics}
and~\ref{fig:interaction_semantics}) and projection/extraction (see
Fig.~\ref{fig:proj_extr}). We present concrete, representative cases
for each of these tranformations. The remaining cases are obtained in
a similar manner.

\subsection{Commuting conversions}
\label{sec:app-commconv}
The majority of the rules for structural
equivalence are derived from the proof of cut-elimination for linear
logic. The deconstruction of the $\m{Cut}$ rule into $\m{Conn}$ and
$\m{Scope}$ results in an altered structural equivalence relation:
instead of permuting applications of $\m{Cut}$ with rules applicable
directly before (or after) it in the proof tree, we have two sets of
such permutations -- one for $\m{Conn}$ and one for
$\m{Scope}$. Intuitively, applications of $\m{Conn}$ and $\m{Scope}$
have to meet before they can be eliminated. As we are interested only
in commuting conversions of typeable programs, there are certain cases
where the correct equivalence can be found only by looking at the
typing derivation. For instance, a choice between rules ${(\gensend)
  \pp \til S} \equiv {\send{x}{x'}{y',\til z'}{(P\pp \til S)}{Q}}$ and
${(\gensend) \pp \til S} \equiv {\send{x}{x'}{y',\til z'}{P}{(Q \pp
    \til S)}}$ follows from two possible origins of the endpoint
getting connected via $\m{Conn}$. In each concrete case precisely one
of the available options will typecheck. As an example, consider the
following proof derivation:
\[\scriptsize
\infer{\judge{\Sigma}
  {(\send x x' P Q) \pp (S_i)_i}
  {(\Phi_i)_i \pp \Phi_P \pp \Phi_Q \pp (\seq \Gamma_i, \pair{x_i}{A_i})_i \pp
    \seq \Gamma_P, \Gamma_Q, \pair{x}{A\tensor B},\pair{z}{C}}}
  {\infer{\judge{\Sigma_P, \Sigma_Q}{\send x x' P Q}{\Phi_P \pp \Phi_Q \pp \seq \Gamma_P, \Gamma_Q, \pair{x}{A \tensor B}, \pair{z}{C}}}
        {\mathcal{D_P} & 
          \mathcal{D}_Q} &
        {\left(\mathcal{D}_i\right)_i}  &
        {\mathcal{D_G}}} 
  \]
  with
  \[\begin{array}{l}
\left(\mathcal{D}_i :: \judge{\Sigma_i}{S_i}{\Phi_i \pp \seq \Gamma_i, \pair{x_i}{A_i}}\right)_i\\
\mathcal{D}_P ::\judge{\Sigma_P}{P}{\Phi_P \pp \Gamma_P, \pair{x'}{A}, \pair{z}{C}}\\
\mathcal{D}_Q ::\judge{\Sigma_Q}{Q}{\Phi_Q \pp \Gamma_Q, \pair{x}{B}}\\
\mathcal{D}_G :: G \gseq (\pair{x_i}{A_i})_i, \pair z C\\
\Sigma = (\Sigma_i)_i, \Sigma_P, \Sigma_Q,\pair{(x_i)_i z}{G}
\end{array}\]
      
Here, the endpoint $z$ used for connecting $\gensend$ to $(S_i)_i$
originates from the hypersequent of $P$ (note that it could also have
been in another sequent from $\Phi_P$, not only -- as is considered
above -- in the same sequent as $x'$; this does not change the
commuting conversion rule). Equivalently, we can give the following
derivation:
\[\scriptsize
\infer{\judge{\Sigma}
  {\send{x}{x'}{y',\til z'}{(P\pp (S_i)_i))}{Q}}
  {(\Phi_i)_i \pp \Phi_P \pp \Phi_Q \pp (\seq \Gamma_i, \pair{x_i}{A_i})_i \pp
    \seq \Gamma_P, \Gamma_q, \pair{x}{A\tensor B},\pair{z}{C}}}
      {\infer{\judge{(\Sigma_i)_i, \Sigma_P,\pair{(x_i)_i z}{G}}{P\pp (S_i)_i}
          {(\Phi_i)_i \pp \Phi_P \pp (\seq \Gamma_i, \pair{x_i}{A_i})_i \pp
    \seq \Gamma_P, \pair{x'}{A},\pair{z}{C}}}
        {{\mathcal{D_P}} &
          \left({\mathcal{D}_i}\right)_i &
        {\mathcal{D_G}}} &
        {\mathcal{D}_Q}}
      \]

This yields one of the rules for commuting conversions: ${(\gensend)
  \pp \til S} \equiv {\send{x}{x'}{y',\til z'}{(P\pp \til
    S)}{Q}}$. Had $z$ be in the hypersequent of $Q$, the other case
would have been chosen.

Next, we observe that there is no commuting conversion between
$\m{Conn}$ and $\bang $. Indeed, to introduce a $\gensrv$ we need to
know that that nothing is connected to $P$. Therefore, in the
interaction fragment, we only allow this commuting conversion if the
endpoint taking part in the connection originated from a different
sequent, than the endpoint of the server type. Of course, in order to
obtain a deadlock freedom result, we need to have \emph{some}
commuting conversion for $\gensrv$ -- it is, for this system, a
slightly unusual one, as we commute $\bang $ introduction past both
$\m{Conn}$ and $\m{Scope}$:
\[ \scriptsize
\infer{\judge{}{\res{{\til x x}:\!G}(\gensrv \pp \til Q)}{\seq \quest
    \Gamma, \left(\quest \Gamma_i\right)_i, \pair y{\bang A}}}
      {\infer{\judge{\pair{(\til x, x)}{G}}{\gensrv \pp \til Q}{\seq
            \Gamma, \pair x{\quest B}, \pair y{\bang A} \pp \left(
            \seq \quest \Gamma_i, \pair{x_i}{B_i}\right)_i}}
        {\infer{\judge{}{\gensrv}{\seq \quest \Gamma, \pair x{\quest
                B}, \pair y{\bang A}}} {\deduce{\judge{}{P}{\seq \quest
              \Gamma, \pair x{\quest B}, \pair y A}}{\mathcal{D}_P}}&
          \left(\deduce{\judge{}{Q_i}{\seq \quest \Gamma_i,
              \pair{x_i}{B_i}}}{\mathcal{D}_i}\right)_i&
          \deduce{G \gseq \left(\pair{x_i}{B_i}
          \right)_i, \pair{x}{\quest B}}{\mathcal{D}_G}}}
  \]

  becomes
  
\[\scriptsize
\infer{\judge{}{\srv{y}{}{\res{{\til x x}:\!G}(P \pp \til Q)}}{\seq \quest \Gamma, \left(\quest \Gamma_i\right)_i, \pair y{\bang A}}}
      {\infer{\judge{}{\res{{\til x x}:\!G}(P \pp \til Q)}{\seq \quest \Gamma, \left(\quest \Gamma_i\right)_i, \pair y{A}}}
        {\infer{\judge{\pair{(\til x, x)}{G}}{P \pp \til Q}{\seq \Gamma, \pair x{\quest B}, \pair y{A} \pp \left( \seq \quest \Gamma_i, \pair{x_i}{B_i}\right)_i}}
        {\deduce{\judge{}{P}{\seq \quest \Gamma, \pair x{\quest B}, \pair y A}}{\mathcal{D}_P}&
          \left(\deduce{\judge{}{Q_i}{\seq \quest \Gamma_i, \pair{x_i}{B_i}}}{\mathcal{D}_i}\right)_i&
          \deduce{G \gseq \left(\pair{x_i}{B_i} \right)_i, \pair{x}{\quest B}}{\mathcal{D}_G}}}}
      \]
        
This proof tranformation gives rise to a commuting conversion of the shape
$\res{{\til x x}:\!G}(\gensrv \pp \til Q) \equiv \srv{y}{}{\res{{\til
      x x}:\!G}(P \pp \til Q)}$ -- but only in the case when a
connection is made with processes which are not connected to anything,
and whose endpoints are of $\quest$ type. This is enough for our
purposes, and is in fact a generalization of the standard commuting
conversion for $\bang$, as found in \cite{W14}. In the interaction
fragment we require the same of the connecting $Q_i$s, giving rise to
the commuting conversion: $\res{{\til z z}:\!G}(\gengclone \pp \til Q)
\equiv \gclone x{\til y}{x'}{\til y'}{\res{{\til z z}:\!G}(P\pp\til
  Q)}$. A similar situation arises again when considering $\top$: we
can only permute $\top$ with both $\m{Conn}$ and $\m{Scope}$ at once,
and only if the connecting processes are themselves not connected to
anything. This is consistent with the process interpretation: within
this session, an empty choice is offered, forcing the communication to
cease:
\[\scriptsize
\infer{\judge{}{\res{{\til z,z}:\!G}{(\nocase{x}{}{\til u, z}\pp \til Q)}}{\seq \Gamma, \left(\Gamma_i\right)_i, \pair{x}{\top}}}
      {\infer{\judge{\pair{(\til z, z)}{G}}{\nocase{x}{}{\til u, z}\pp \til Q}{\seq \Gamma, \pair{x}{\top}, \pair{z}{B} \pp \left(\seq \Gamma_i, \pair{z_i}{B_i} \right)_i}}
        {\infer{\judge{}{\nocase{x}{}{\til u, z}}{\seq \Gamma,\pair{z}{B},\pair{x}{\top}}}
          {\m{vars}(\Gamma) = \til u} &
          \left(\deduce{\judge{}{Q_i}{\seq \Gamma_i, \pair{z_i}{B_i}}}{\mathcal{D}_i} \right)_i &
            \deduce{G \gseq \left(\pair{z_i}{B_i}\right)_i, \pair{z}{B}}{\mathcal{D}_G}}}
\]
becomes
\[\scriptsize
\infer{\judge{}{\nocase{x}{}{\til u, \til v}}{\seq \Gamma, \left(\Gamma_i\right)_i, \pair{x}{\top}}}
{\m{vars}(\Gamma) = \til u & \left(\m{vars}(\Gamma_i)\right)_i = \til v}
\]
The commuting conversion in this case is $\res{{\til
    z,z}:\!G}{(\nocase{x}{}{\til u, z}\pp \til Q)} \equiv
{\nocase{x}{}{\til u, \til v}}$ where $\til v = \m{vars}(\til Q) \setminus \til z$

\subsection{Reductions}
\label{sec:app-reductions}
To provide intuition about the semantics coming
from cases of $\m{Scope}$ elimination in our system, we show a proof
transformation in the case of session creation.

\[\scriptsize
\infer
      {\judge
        {\Sigma}
        {{{\res {\til xy {\til z} : \gcom{\til x}{y}{G};H} \gencom}}}
        {\Psi \pp \seq (\Gamma_{i1}, \Gamma_{i2})_i, \Gamma, (\Gamma_j')_j}}{
\infer
      {
        \judge{\Sigma,{\pair{(\til x,y,\til z)}{\gcom{\til x}{y}{G};H}}}
              {{\gencom}}
              {
                \Psi
                \pp
                {( \seq \Gamma_{i1},\Gamma_{i2}, \pair{x_i}{A_i \tensort y B_i} )_i} \pp
                \seq \Gamma, {\pair{y}{C \parrt{\til x} D} \pp
                {( \seq \Gamma'_{j}, \pair{u_j}{E_j} )_j}}
              }
      }
      {\deduce{
        \judge{\Sigma,{\pair{(\til x, y, \til z)}{H},\pair{(\til x',y')}{G\{\til x'/\til x,y'/y\}}}}
              {{P}}
              {
                \Psi
                \pp
                {( \seq \Gamma_{i1}, \pair{x'_i}{A_i} )_i \pp
                  ( \seq \Gamma_{i2}, \pair{x_i}{B_i} )_i} \pp
                \seq \Gamma, {\pair{y'}{C}, \pair{y}{D} \pp
                {( \seq \Gamma'_{j}, \pair{u_j}{E_j} )_j}}
              }
      }{\mathcal{D}}}
      }
      \]
      becomes
\[\scriptsize \infer
      {\judge
        {\Sigma}
        {{\res{\til x'y' : G\{\til x'/\til x,y'/y\}} \res{\til xy {\til z} : H} P}}
        {\Psi \pp \seq (\Gamma_{i1}, \Gamma_{i2})_i, \Gamma, (\Gamma'_j)_j}
      }
    {\infer
      {\judge{\Sigma,\pair{(\til x',y')}{G\{\til x'/\til x,y'/y\}}}
        {\res{\til xy {\til z} : H} P}
        {\Psi \pp (\seq \Gamma_{i1}, x'_i:A_i)_i\pp \seq \Gamma,\pair{y'}{C},(\Gamma_{i2})_i,(\Gamma'_j)_j }}
      {\deduce{
        \judge{\Sigma,{\pair{(\til x, y, \til z)}{H},\pair{(\til x',y')}{G\{\til x'/\til x,y'/y\}}}}
              {{P}}
              {
                \Psi
                \pp
                {( \seq \Gamma_{i1}, \pair{x'_i}{A_i} )_i \pp
                  ( \seq \Gamma_{i2}, \pair{x_i}{B_i} )_i} \pp
                \seq \Gamma, {\pair{y'}{C}, \pair{y}{D}\pp
                {( \seq \Gamma'_{j}, \pair{u_j}{E_j} )_j}}
              }
      }{\mathcal{D}}}}
    \]
    This justifies the reduction:
    \[{\gcpres{\til x, y, \til z}
      {\gcom{\til x}{y}{G};H}
      { \left(\gencom\right) }}
     \reducesto
     {\gcpres{\til x', y'}
      {G\{\til x'/\til x,y'/y\}} {\gcpres{\til x, y, \til z}{H}
        {P}}}\]

\subsubsection{Server Cloning}
\label{sec:app-cloning}

When a client process requests a server to clone ($\genclone$), or
when cloning of the server is part of the choreography ($\gengclone$),
the semantic rules governing the execution of such a system have to
ensure certain enpoints get connected at the server-side.

At a proof system level, this is because the weakening in the
exponential fragment is not trace-free. It is worth looking at the
proof transformations that give rise to the semantic rules we have
obtained:
\[\scriptsize
\infer
    {\judge{\Sigma}{\gcpres{x, \til y}{\gbang{x}{\til y}{G}} \genclone \pp (\srv{y_i}{x}{Q_i})_i}{\Psi \pp \seq \Gamma, (?\Gamma_i)_i}}
    {\infer{\judge{\Sigma, (x, \til y) : \gbang{x}{\til y}{G}}{\genclone \pp (\srv{y_i}{x}{Q_i})_i}{\Psi \pp \seq \Gamma, x : ?A \pp (\seq ?\Gamma_i, y_i : !B_i)_i}}
      {\mathcal{D}_G &
        \infer{\judge{\Sigma}{\genclone}{\Psi \pp \seq \Gamma, x : ?A}}
              {\mathcal{D}_P} &
        \left({\mathcal{D}_i}\right)_i
      }}
    \]
    where
    \[
    \begin{array}{l}
      \mathcal{D}_G = {\infer{\gbang{x}{\til y}{G} \gseq x: ?A, (y_i: !B_i)_i}{\deduce{G \gseq x : A, (y_i:B_i)_i}{...}}}\\[3mm]
      \mathcal{D}_P :: \judge{\Sigma}{P}{\Psi \pp \seq \Gamma, x : ?A, x' : ?A}\\[3mm]
      \mathcal{D}_i = \infer{\judge{}{\srv{y_i}{x}{Q_i}}{\seq ?\Gamma_i, y_i : !B_i}}{\deduce{\judge{}{Q_i}{\seq ? \Gamma_i, y_i : B_i}}{...}}
    \end{array}
    \]
becomes 
\[\tiny 
\infer{\judge{\Sigma}{(\cloneo{u_j}{u_j'})_j; \gcpres{x, \til y}{\gbang{x}{\til y}{G}}
        {\gcpres{x', \til y'}{\gbang{x'}{\til y'}{G'}}
          {P \pp (\srv{y_i}{x}{Q_i})_i} \pp (\srv{y'_i}{x'}{Q_i'})_i}}{\Psi \pp \seq \Gamma, (?\Gamma_i)_i}}
{\infer{\judge{\Sigma}{\gcpres{x, \til y}{\gbang{x}{\til y}{G}}
        {\gcpres{x', \til y'}{\gbang{x'}{\til y'}{G'}}
          {P \pp (\srv{y_i}{x}{Q_i})_i} \pp (\srv{y'_i}{x'}{Q_i'})_i}}{\Psi \pp \seq \Gamma, (?\Gamma_i)_i, (?\Gamma'_i)_i}}
  {\infer{
      \judge
          {\Sigma, ({x, \til y}) : {\gbang{x}{\til y}{G}}}
          {\gcpres{x', \til y'}{\gbang{x'}{\til y'}{G'}}
            {P \pp (\srv{y_i}{x}{Q_i})_i} \pp (\srv{y'_i}{x'}{Q_i'})_i}
          {\Psi \pp \seq \Gamma, (?\Gamma'_i)_i, x : ?A \pp (\seq \Gamma_i, y_i:!B_i)_i}}
  {\infer{\judge{\Sigma, (x, \til y) : {\gbang{x}{\til y}{G}}, (x', \til y') : \gbang{x'}{\til y'}{G'}}
    {{P \pp (\srv{y_i}{x}{Q_i})_i} \pp (\srv{y'_i}{x'}{Q_i'})_i}
    {\Psi \pp \seq \Gamma, x:?A, x':?A \pp (\seq \Gamma_i, y_i : !B_i)_i \pp (\seq \Gamma'_i, y'_i : !B_i)_i }}
    {\mathcal{D}_G      &
      \infer{\judge{\Sigma, (x', \til y') : {\gbang{x'}{\til y'}{G'}}}{P \pp (\srv{y_i'}{x'}{Q_i'})_i}{\Psi \pp \seq \Gamma, x:?A, x':?A \pp (\seq\Gamma'_i, y_i':!B_i)_i}}
            {\mathcal{D}_{G}'
              & \mathcal{D}_P
              & \left(\mathcal{D}_i'\right)_i}
      &
      \left(\mathcal{D}_i\right)_i
      }}}}
\]

with the following conventions
\[\begin{array}{l}
G' = G\{x'/x,\til y'/\til y\}\\[3mm]
\mathcal{D}_{G}' = {\infer{\gbang{x'}{\til {y'}}{G} \gseq x': ?A, (y_i': !B_i)_i}
  {\deduce{G \gseq x : A, (y_i':B_i)_i}{...}}} \\[3mm]
\mathcal{D}_i' = \infer{\judge{}{\srv{y_i'}{x'}{Q'_i}}{\seq \Gamma'_i, y'_i : ! B_i}}
        {\deduce{\judge{}{Q'_i}{\seq \Gamma'_i, y_i' : B_i}}{...}}
\end{array}\]
  
and assuming $\forall j . \exists i . u_j \in \Gamma_i \wedge u'_j \in \Gamma'_i$.

This gives rise to the semantic rule
${\gcpres{x, \til y}{\gbang{x}{\til y}{G}} \big(\genclone \pp (\srv{y_i}{x}{Q_i})_i\big)}
\reducesto$\\
$ {\left(\cloneo{u_j}{u_j'}\right)_j; \gcpres{x, \til y}{\gbang{x}{\til y}{G}}
        {\gcpres{x', \til y'}{\gbang{x'}{\til y'}{G\{x'/x,\til y'/\til y\}}}
          {\big(P \pp (\srv{y_i}{x}{Q_i})_i} \pp (\srv{y'_i}{x'}{Q_i'})_i\big)}}$.

\subsection{Projection/extraction}
\label{sec:app-projextr}
Finally, the justification for the shape of the rules for extraction
$\extr$ and projection $\proj$ can be given in terms of proof
transformations. We will focus on justifying the rewrite rules for
communication:
\[\left(\send{x_i}{x_i'}{y',\til x'_{\setminus
    i}}{P_i}{Q_i}\right)_i \pp \recv{y}{\til x'}{y'}R \pp \til S
\quad\projextr\quad \com{\til x}{\til x'}{y}{y'}{\left(\til P \pp \til
  Q\pp R \pp \til S\right)}\]

First, the typing derivation for the left-hand side is presented on
Fig.~\ref{fig:projextr_ex1}. Here we begin by send and receive
operations, which are then followed by a connection to the remainder
of the participants in $\til S$. However, we can reorder these two
operations; knowing:
\[\infer{\gcom{\til x}{y}{G};H \gseq (x_i:A_i\tensor B_i), y:C\parr D, (z_j:A_j)_j}
        {\deduce{G \gseq (x_i:A_i)_i,y:C}{\mathcal{D}_G} & \deduce{H \gseq(x_i:B_i)_i, y:D, (z_j:A_j)_j}{\mathcal{D}_H}}
\]
we can first connect $\til x$ with $y$ and, separately,
$\til x, y, \til z$ into two sessions, which can then be composed
using the choreographic communication rule, as presented on
Fig.~\ref{fig:projextr_ex2}.
        
\begin{sidewaysfigure}  
  \[\tiny
\infer
  {
    \judge{(\Sigma_j)_j,(\Sigma_{i_1},\Sigma_{i_2})_i,\Sigma_R,\pair{(\til x,y,\til z)}{\gcom{\til x}{y}{G};H}}
          {\left(\send{x_i}{x_i'}{}{P_i}{Q_i}\right)_i \pp
            \recv{y}{\til x'}{y'}R \pp
            \til S}
          {
            (\Psi_j)_j\pp(\Psi_{i_1}\pp\Psi_{i_2})_i\pp\Psi_R
            \pp
            \left(\seq \Gamma_j, z_j : A_j\right)_j \pp
            \left( \seq \Gamma_{i_1},\Gamma_{i_2}, \pair{x_i}{A_i \tensort y B_i} \right)_i \pp
            \seq \Gamma_R, \pair{y}{C \parrt{\til x} D}
      }
  }
  {
    ({\mathcal{D}_j})_j &
    \left(\infer{
      \judge{(\Sigma_{i_1},\Sigma_{i_2})_i}
        {\send{x_i}{x_i'}{}{P_i}{Q_i}}
        {
          (\Psi_{i_1}\pp\Psi_{i_2})_i
          \pp
          \seq \Gamma_{i_1},\Gamma_{i_2}, \pair{x_i}{A_i \tensort y B_i} 
        }}
    {
      \deduce{\judge{\Sigma_{i_1}}{P_i}{\Psi_{i_1} \pp \seq\Gamma_{i_1},\pair{x'_i}{A_i}}}{\mathcal D_{i_1}}
      &
      \deduce{\judge{\Sigma_{i_2}}{Q_i}{\Psi_{i_2} \pp \seq\Gamma_{i_2},\pair{x_i}{B_i}}}{\mathcal D_{i_2}}
    }\right)_i
    &
    \infer{
      \judge{\Sigma_R}
        {\recv{y}{\til x'}{y'}R}
        {
          \Psi_R
          \pp
          \seq \Gamma_R, \pair{y}{C \parrt{\til x} D}
        }
    }
    {
      \deduce{\judge{\Sigma_R}{R}{\seq \Gamma_R, \pair{y'}{C}, \pair{y}{D}}}{\mathcal{D}_R}
    }
    &
    \mathcal{D}_{GH}
  }
  \]
  with \[\begin{array}{l}
  \mathcal{D}_j = \deduce{\judge{\Sigma_j}{S_j}{\Phi_j \pp \Gamma_j, y_j : A_j}}{...}\\[2mm]
  \mathcal{D}_{GH} = \infer{\gcom{\til x}{y}{G};H \gseq (x_i:A_i\tensor B_i), y:C\parr D, (z_j:A_j)_j}
          {\mathcal{D}_G & \mathcal{D}_H}\\[2mm]
          \mathcal{D}_G ::  G' \gseq (x_i':A_i)_i, y: C\\[2mm]
\mathcal{D}_H :: H \gseq (x_i:B_i)_i, y: D, (z_j:A_j)_j

  \end{array}\]
      \caption{Example typing derivation: first send/receive, then connect.}
  \label{fig:projextr_ex1}
\end{sidewaysfigure}
\begin{sidewaysfigure}
\[\tiny
\infer
  {
    \judge{(\Sigma_j)_j,(\Sigma_{i_1},\Sigma_{i_2})_i,\Sigma_R,\pair{(\til x,y,\til z)}{\gcom{\til x}{y}{G};H}}
      {\com{\til x}{\til x'}{y}{y'}{\left(\til P \pp \til Q \pp R\pp\til S\right)}}
      {
        (\Psi_j)_j\pp(\Psi_{i_1}\pp\Psi_{i_2})_i\pp\Psi_R
        \pp
        \left(\seq \Gamma_j,z_j:A_j\right)_j\pp
        \left( \seq \Gamma_{i_1},\Gamma_{i_2}, \pair{x_i}{A_i \tensort y B_i} \right)_i \pp
        \seq \Gamma_R, \pair{y}{C \parrt{\til x} D}
      }
  }
  {
    \infer
      {
        \judge{(\Sigma_j)_j,(\Sigma_{i_1},\Sigma_{i_2})_i,\Sigma_R,\pair{(\til x, y, \til z)}{H},\pair{(\til x',y')}{G'}}
          {\til P \pp \til Q \pp R \pp \til S}
          {
            (\Psi_j)_j \pp (\Psi_{i_1}\pp\Psi_{i_2})_i\pp\Psi_R
            \pp
            \left(\seq \Gamma_j, \pair{z_j}{A_j}\right)_j\pp
            \left( \seq \Gamma_{i_1}, \pair{x'_i}{A_i} \right)_i \pp
            \left( \seq \Gamma_{i_2}, \pair{x_i}{B_i} \right)_i \pp
            \seq \Gamma_R, \pair{y'}{C}, \pair{y}{D}
          }
      }
      {\left(\deduce{\judge{\Sigma_{i_1}}{P_i}{\Psi_{i_1} \pp \seq\Gamma_{i_1},\pair{x'_i}{A_i}}}{\mathcal D_{i_1}}\right)_i &
        \infer
          {
            \judge{(\Sigma_j)_j, (\Sigma_{i_2})_i,\Sigma_R,\pair{(\til x,y,\til z)}{H}}
              {(Q_i)_i\pp R \pp \til S}
              {(\Psi_j)_j \pp (\Psi_{i_2})_i \pp
                (\seq \Gamma_j, \pair{z_j}{A_j})_j \pp
                (\seq \Gamma_{i_2},\pair{x_i}{B_i})_i \pp
                \seq \Gamma_R, \pair{y'}{C}, \pair{y}{D}
              }
          }
          {\left(\mathcal{D}_j\right)_j &
            \left(\deduce{\judge{\Sigma_{i_2}}{Q_i}{\Psi_{i_2} \pp \seq\Gamma_{i_2},\pair{x_i}{B_i}}}{\mathcal D_{i_2}}\right)_i &
            \deduce{\judge{\Sigma_R}{R}{\seq \Gamma_R, \pair{y'}{C}, \pair{y}{D}}}{\mathcal{D}_R}
            &
            \mathcal{D}_H
          }
          &
         \mathcal{D}_G
      }
  }
\]   
with \[\begin{array}{l}
G' = G\{\til x'/\til x,y'/y\}\\[2mm]
\end{array}\]
  \caption{Example typing derivation: first connect, then send/receive.}
  \label{fig:projextr_ex2}
\end{sidewaysfigure}

%%% Local Variables: 
%%% mode: latex
%%% TeX-master: "main"
%%% End: 
